# Supplementary material for: 3DMorph: Single-Image-Guided Local 3D Shape Editing and Morphing
Source: arXiv:2606.07115 source file (2026-06-05)
Supplement: Supplementary file 1 [file BB-pred-influence.tex]

\textbf{Bounding box prediction.} Fig.~\ref{fig:BB-influence} evaluates the effect of bounding box prediction quality on editing performance. We measure quality using Intersection over Ground Truth (IoGT) between the predicted and ground-truth boxes. IoGT prioritizes coverage of the target region over penalizing extra area. On average, the predicted boxes achieve an IoGT slightly below 60\%. To further analyze the influence of the prediction module, we compare 3DMorph and 3DMorph-BB under varying IoGT thresholds by filtering out low-quality predictions. As bounding box quality improves, the performance gap between the two variants diminishes, underscoring the importance of precise localization.

% --- size knobs ---
\newcommand{\panelW}{0.25\textwidth} % width of each subplot
\newcommand{\panelH}{4cm}          % height of each subplot
\newcommand{\panelSep}{30pt}          % horizontal gap between subplots

\begin{figure*}
\begin{tikzpicture}
\begin{groupplot}[
  myaxis,
  width=\panelW,
  height=\panelH,
  group style={group size=3 by 1, horizontal sep=\panelSep},
  tick label style={font=\small},
  label style={font=\small},
  title style={font=\small},
]

% --- (1) CD (down) ---
\nextgroupplot[
  title={$CD\:\downarrow$},
  ymin=0.020, ymax=0.032,
  grid=both, minor tick num=1, tick align=outside,
  legend pos=north east
]
\addplot[mark=*, color=Morph, thick] coordinates {(all,0.0301) (0.3,0.0263) (0.5,0.0244) (0.7,0.0230) (0.9,0.0217)};
\addplot[mark=o, color=MorphBB, thick] coordinates {(all,0.0230) (0.3,0.0217) (0.5,0.0215) (0.7,0.0207) (0.9,0.0213)};
\legend{3DMorph, 3DMorph-BB}

% --- (2) IoU (%) (up) ---
\nextgroupplot[
  title={$IoU\:(\%)\:\uparrow$},
  ymin=59, ymax=68,
  grid=both, minor tick num=1, tick align=outside,
  legend pos=south east
]
\addplot[mark=*, color=Morph, thick] coordinates {(all,60.29) (0.3,61.92) (0.5,62.90) (0.7,64.04) (0.9,65.40)};
\addplot[mark=o, color=MorphBB, thick] coordinates {(all,65.17) (0.3,65.98) (0.5,66.04) (0.7,66.64) (0.9,65.56)};
\legend{3DMorph, 3DMorph-BB}

% --- (3) left axis: SAMPLES as bars (shift left) ---
\nextgroupplot[
  title={BB-IoGT + \#Samples},
  ybar,
  bar width=6pt,            % <- keep same on BOTH axes
  enlarge x limits=0.18,     % <- same padding on BOTH axes
  ymin=0, ymax=900,
    ymajorgrids,                % <--- add horizontal grid lines
    grid style={dashed,gray!50}, % <--- style of the grid
  legend pos=north west
]
\addplot+[fill=gray, draw=gray, bar shift=-6pt] coordinates {
  (all,816)
  (0.3,650)
  (0.5,527)
  (0.7,306)
  (0.9,132)
};
\addlegendentry{Samples}

\end{groupplot} % <--- close the group BEFORE overlaying

% --- Overlay RIGHT y for panel (c3r1): BB-IoGT as bars (shift right) ---
\begin{axis}[
  myaxis,
  width=\panelW,
  height=\panelH,
  at={(group c3r1.center)}, anchor=center,
  axis y line*=right,
  axis x line=none,
  ybar,
  bar width=6pt,            % <- SAME as above
  enlarge x limits=0.18,     % <- SAME as above
  yticklabel style={color=orange},
  y label style={color=orange},
  ymin=0, ymax=1.0,          % bars should start at 0 for bar charts
  trim axis left, trim axis right,
  clip=false,
    ymajorgrids,                % <--- add horizontal grid lines
    grid style={dashed,orange!50} % <--- style of the grid
]
\addplot+[fill=orange, draw=orange, bar shift=+6pt, fill opacity=0.45] coordinates {
  (all,0.5717)
  (0.3,0.688)
  (0.5,0.7574)
  (0.7,0.8817)
  (0.9,0.991)
};
\addlegendentry{BB-IoGT}
\end{axis}

\end{tikzpicture}
\caption{Influence of the bounding box. TOOD.}
\label{fig:BB-influence}
\end{figure*}
